# Supplementary material for: Tight Cutoffs for Guarded Protocols with Fairness
Source: arXiv:1505.03273 source file (2015-11-05)
Supplement: Supplementary file 1 [file appendix1.tex]

\subsection{Undecidability of Template Synthesis}
\sj{Optional, not sure about proof}\ak{if not sure lets remove and add into camera-ready, may also put it as a conjecture}
Checking realizability of LTL
specifications has been shown to be undecidable for architectures in
which processes have incomparable information about the environment 
in the synchronous case~\cite{Finkbeiner05}, and even for
all architectures with more than one system process in the
asynchronous case~\cite{Schewe06}.

Even though we reduce the parameterized template synthesis problem to a template synthesis problem with fixed multiplicity, the problem remains undecidable:

\begin{thm}
\label{thm:undecidable-synthesis}
The template synthesis problem is undecidable for specifications in $\LTLmX$ and disjunctive or conjunctive process templates.
\end{thm}

\begin{proof}
The undecidability proof for distributed synthesis of synchronous processes 
by Pnueli and Rosner~\cite{Rosner92} can be modified to work for this 
restricted class of systems and specifications (cp. also ~\cite{Jacobs14} and 
~\cite{Schewe13} for similar modifications of the proof). The proof develops 
a specification that requires both processes to simulate a Turing machine $M$
, and terminate. Thus, solving the synthesis problem would solve the halting 
problem. 

There are essentially two problems that need to be solved to make the 
original proof work: i) processes can observe the state of each other, and ii)
 our specification is restricted to $\LTLmX$. To solve problem i), we use the 
interleaving semantics of our systems, and force each process to return to a 
``neutral'' state after the simulation of one step of $M$. Thus, when the 
other process is scheduled, it will gain no information about the progress of 
the other. To solve problem ii), we modify the specification such that next-
state subformulas are replaced with formulas referring to the next time the 
process leaves its neutral state.
\end{proof}
 
%An LTS $(T,t_0,\delta,o)$ \emph{satisfies} an LTL formula $\spec$ if, for all
%infinite sequences $(t^0,e^0),(t^1,e^1),\ldots$, where $t^0 = t_0$, $e^i \subs%eteq O_{env}$ and
%$t^{i+1} = \delta(t^i,e^i)$, 
%the sequence $\sigma: i \mapsto o(t^i) \cup e^i$ is a model of $\spec$.

%
%\subsubsection*{Asynchronous Systems.} An \emph{asynchronous system} is an LTS such that
%in every transition, only a subset of the system processes changes their
%state. This is decided by a \emph{scheduler} that can choose for every
%transition which of the processes (including the environment) is allowed to make a step. In
%our setting, we will assume that the environment is always scheduled, and
%consider the scheduler as a part of the environment.
%
%Formally, $O_{env}$ contains additional scheduling
%variables $s_1, \ldots, s_k$, and $s_i \in I_i$ for every $i$. For any
%$i \in P^-,t \in T_i$ and $I \subseteq I_i$, we require $\delta_i(t,I) = t$ whenever $s_i \not \in I$.

%We assume that guarded protocols are implemented with interleaving semantics, i.e., in every step only one system process may change its state. 
%This means that in contrast to inputs from the
%  environment, an input $\send_i$ implies that the receiving process is also
%  scheduled.
%We only consider executions in which scheduling and token-passing is fair.
